# Supplementary material for: High-Temperature Non-Equilibrium Atom-Diatom Collisional Energy Transfer
Source: arXiv:2409.08955 source file (2024-09-13)
Supplement: Supplementary file 1 [file N3_SM_20240723.pdf]

SUPPLEMENTAL MATERIAL

JULY 23, 2024

# High-Temperature Non-Equilibrium Atom-Diatom Collisional Energy Transfer

Xiaorui Zhao[1,2], Xuefei Xu[1,3,*], and Haitao Xu[1,2,*]

[1] *Center for Combustion Energy, Tsinghua University, Beijing 100084, P. R. China*

[2] *School of Aerospace Engineering, Tsinghua University, Beijing 100084, P. R. China*

[3] *Department of Energy and Power Engineering, Tsinghua University, Beijing 100084, P. R. China*

*Corresponding authors: xuxuefei@tsinghua.edu.cn, hxu@mail.tsinghua.edu.cn

# Content

1. **Quasi-Classical Trajectory Simulation ........................................................4**

2. **State-to-State Transition Rate Coefficients ..................................................6**

3. **Semi-Analytical Model for Transition Rate Coefficients ............................9**

4. **Relaxation of $N$+$N_2$ after Passing a Shock in Hypersonic Flows.............15**

In the supplemental material, we provide some details of computational methods, as well as additional results and discussions. In section 1, we first provide a brief introduction of quasi-classical trajectory (QCT) simulation, then introduce the systems studied in current work and their potential energy surfaces. The ro-vibrational states involved in our studied $N+N_2$ system are introduced, and some simulation setting details are also provided. In section 2, we introduce how to calculate the state-to-state transition rate coefficients from batches of trajectories, and our calculated results are presented and compared with some theoretical and empirical models. Here the wide range vibrational energy transfer is found to be significant in high temperature, however underestimated in previous work, which inspired us to investigate further. In section 3, some details of our proposed Activation-Saturation (AS) model are introduced. We found a universal “activation-saturation”-like behavior of the transition probability with collision energy, based on which a general analytical model is proposed, shown in subsection 3.1. Furtherly we derivate the analytical form of rate coefficients calculation using the steepest descent integration, and the mathematical details are shown in subsection 3.2. In subsection 3.3, the results of rate coefficients from our AS model are presented, which agree well with the original QCT data. In subsection 3.4, we demonstrate the results of other atom-diatom systems, which also have the consistent “activation saturation”-like behavior. In section 4, to evaluate our proposed model, some examples of the vibrational energy relaxation of $N+N_2$ after passing strong shocks in hypersonic flows are given. We first introduce the master equation approach briefly, based on which the evolution of the vibrational energy distribution can be solved. Our results are presented and compared with available data, including: (4.1) change of vibrational energy with time, (4.2) the relationship of the vibrational relaxation time with translational temperature, and (4.3) the evolution of vibrational energy distribution. In these respects, our results are both in good agreement with the available data. Finally, a brief summary is concluded.

# 1. Quasi-Classical Trajectory Simulation

The quasi-classical trajectory (QCT) method is widely used in simulating molecular collision [1–3], and surface scattering [4,5], et. al., in which the initial/final states of molecules are specified into quantum states, and the dynamics is treated classically solved with Hamilton's equations:

$$\frac{d\boldsymbol{Q}}{dt}=\frac{\partial H}{\partial \boldsymbol{P}} \tag{S1 − 1}$$

$$\frac{d\boldsymbol{P}}{dt}=-\frac{\partial H}{\partial \boldsymbol{Q}} \tag{S1 − 2}$$

in which, $\boldsymbol{Q}$ and $\boldsymbol{P}$ are the generalized coordinate and generalized momentum of system respectively, $H$ is the classical Hamiltonian of system, that $H=T(\boldsymbol{P})+V(\boldsymbol{Q})$, where $T(\boldsymbol{P})$ and $V(\boldsymbol{Q})$ are kinetic energy and potential energy of system respectively.

In QCT, each trajectory represents the dynamics from a specific initial condition, and the state-to-state transition rates and the reaction rates can be calculated statistically with batches of trajectories (details will be introduced in section 2). When the nuclear mass is large and the energy is high, QCT proves to be a reliable approach with less significant quantum effects [1], therefore it is suitable for molecular simulation in hypersonic flows.

## 1.1 System Studied and Potential Energy Surface

In current work, we mainly simulate $N+N_2$ collision dynamics because nitrogen is the major ingredient of air, thus its energy transfer controls the relaxation of air to equilibrium. Moreover, compared to oxygen, another important ingredient of air, nitrogen has a higher dissociation energy barrier and a higher electronic excitation energy level, making the collisional energy transfer process less affected by dissociation and electronic excitation.

$N+N_2$ dynamics simulation is based on a recently reported high accuracy *ab initio* potential energy surface (PES) for the $N_3$ $(4A'')$ system ground state which governs electronically adiabatic collisions of $N_2(^1\Sigma_g^+)$ with $N(^4S)$ [6]. For further investigation, we also simulate $O+N_2$ collision dynamics based on the *ab initio* PES for the $N_2O$ $(1^3A'')$ system [7], and $O+O_2$ collision dynamics based on the *ab initio* PES for the $O_3$ $(1^3A'')$ system [8] briefly, and the result are shown in section 3.

## 1.2 Enumeration of Ro-Vibrational States

To generate the ro-vibrational states of $N_2$ diatom molecule, Wenzel-Kramers-Brillouin (WKB) approximation is employed using $N_2$ diatomic potential [6], which is a widely used approach [1,3,9–11]. There are totally 9236 ro-vibrational states, of which 7196 states are bound states (whose energy is lower than the dissociation energy barrier), and 2040 are quasi-bound states (whose energy is higher than the dissociation energy barrier but lower than the *J*-dependent centrifugal barrier). There are 59 vibrational states with vibrational quantum number in the range 0-58, and 284 rotational states with rotational quantum number in the range 0-283.

The vibration-prioritized framework is used to separate the internal energy $E_{\mathrm{int}}$ into vibrational energy $E_{\mathrm{vib}}$ and rotational energy $E_{\mathrm{rot}}$ [3]:

$$E_{\mathrm{vib}}(v,j)=E_{\mathrm{int}}(v,j=0)=E_{\mathrm{vib}}(v) \tag{S1 − 3}$$

$$E_{\mathrm{rot}}(\upsilon, j) = E_{\mathrm{int}}(\upsilon, j) - E_{\mathrm{int}}(\upsilon, j = 0) \quad (\mathrm{S1}-4)$$

In this framework, vibrational energy is the function of only vibrational quantum number $\upsilon$, and rotational energy is the function of both vibrational quantum number $\upsilon$ and rotational quantum number $j$.

## 1.3 QCT Simulation Setting

- Initial condition

In this atom-diatom system, initial coordinates and velocities (or momentums) need to be sampled for trajectory integration. For the $N_2$ molecule, six parameters are needed, including the vibrational quantum number $\upsilon$, the rotational quantum number $j$, the azimuthal orientation angle $\theta$, the polar orientation angle $\phi$, the orientation angle of the angular momentum $\eta$, and the vibrational phase angle $\xi$. For the collision partner N atom, three additional parameters are needed: collision energy $E_{\mathrm{col}}$, cut-off distance $l$ (the separation between the center of mass of the $N_2$ molecule and N atom), and impact parameter $b$ (the eccentric distance between the center of mass of the $N_2$ molecule and N atom). Notice, when the ro-vibrational state $(\upsilon, j)$ of $N_2$ molecule is specified, its vibrational energy and the rotational energy is determined, and further if the collision energy is specified, the total energy of the system is determined.

Because neighboring ro-vibrational states may have similar dynamics characteristics, we just simulated 4 initial vibrational states, with $\upsilon'$=5, $\upsilon'$=15, $\upsilon'$=25, and $\upsilon'$=35 (here we use $'$ to denote the initial state). For each vibrational quantum number, rotational quantum number is sampled with an interval of ten, starting from $j'$=0 to its maximum, totally involving 83 initial ro-vibrational states. 100 collision energies are specified, from 0.1 eV to 10.0 eV with an interval of 0.1 eV.

The cut-off distance is set to 15Å, beyond which the interaction of $N_2$ and N is negligible. The maximum impact parameter is set to 6Å, beyond which the probability of energy transfer and dissociation is negligible. The geometry parameters $(b, \theta, \phi, \eta, \xi)$ are sampled by Monte Carlo method from appropriate probability distribution based on the principle of independent random distribution of $N_2$ and N, more details are given in Ref [1]. For each energy case $(\upsilon', j', E_{\mathrm{col}})$, we run 10000 trajectories, and more than $8\times10^7$ trajectories in total. Convergence for trajectory numbers have been verified.

- Dynamics setting

The 4th order Runge-Kutta method is used to integrate each trajectory with the timestep of 0.05 fs. The trajectory is terminated when any N-N bond length exceed 15Å after collision.

- Software

ANT program [12] was used to implement the QCT initial condition sampling and simulation. This Fortran 90 code has complied with Intel 2017 compiler.

## 2. State-to-State Transition Rate Coefficients

In this section, we introduce how to calculate the state-to-state transition rate coefficients from batches of trajectories, and compare our results with some theoretical and empirical models.

When a trajectory is terminated, there could be two typical outcomes: (i) three separated N atoms, i.e., dissociation event, which could be recognized from the internuclear distances easily; (ii) one N atom with one $N_2$ diatom-molecule, i.e., non-dissociation event, which is the most likely case corresponding to the collisional energy transfer. For non-dissociation events, the final $N_2$ molecules could be specified into ro-vibrational states according to their final configurations and momentum using WKB approximation.

The state-to-state transition probability of $(v', j') \to (v, j)$ transition event with a specific collisional energy $E_{\mathrm{col}}$ could be obtained from a batch of trajectories:

$$P\big((v', j') \to (v, j), E_{\mathrm{col}}\big) = \frac{N\big((v', j') \to (v, j), E_{\mathrm{col}}\big)}{N_{\mathrm{total}}\big((v', j'), E_{\mathrm{col}}\big)} \qquad (\mathrm{S2}-1)$$

We specify the initial ro-vibrational state with $(v', j')$, and the final state with $(v, j)$. On the right hand of Eq. (S2-1), the denominator is the total trajectory numbers in each case, and the numerator is the trajectory numbers of the specific events corresponding to the $(v', j') \to (v, j)$ transition.

Considering all 9000+ ro-vibrational states of the N+$N_2$ system is impossible and not necessary, and the master equation will be intractable to solve with those many states. The commonly used approach is to only take the vibrational states into account, and average the initial rotational states on a given rotational temperature $T_{\mathrm{r}}$, as well as sum over the final rotational states. Therefore, the dependence of rotational quantum number $j'$ and $j$ disappears in the state-to-state transition probability:

$$P(v' \to v, E_{\mathrm{col}}) = \sum_{j}\sum_{j'} g_{\mathrm{B}}(j', v', T_{\mathrm{r}})\, P\big((v', j') \to (v, j), E_{\mathrm{col}}\big) \qquad (\mathrm{S2}-2a)$$

$$g_{\mathrm{B}}(j, v, T_{\mathrm{r}}) = \frac{(2j+1)\exp\left(-\frac{E_{\mathrm{rot}}(v, j)}{k_{\mathrm{B}}T_{\mathrm{r}}}\right)}{\sum_{0}^{j_{\max}(v)}(2j+1)\exp\left(-\frac{E_{\mathrm{rot}}(v, j)}{k_{\mathrm{B}}T_{\mathrm{r}}}\right)} \qquad (\mathrm{S2}-2b)$$

where $g_{\mathrm{B}}(j, v, T_{\mathrm{r}})$ is the weight of ro-vibrational state $(j, v)$ given by the Boltzmann distribution at the rotational temperature $T_{\mathrm{r}}$, and $k_{\mathrm{B}}$ is the Boltzmann constant.

With the state-to-state transition probability, we can obtain the state-to-state transition rate coefficient $k(v' \to v, T)$:

$$k(v' \to v, T) = Z(T)\int_{0}^{\infty} P(v' \to v, E_{\mathrm{col}}) \cdot f_{\mathrm{B}}(E_{\mathrm{col}}, T)\, dE_{\mathrm{col}} \qquad (\mathrm{S2}-3)$$

in which $Z(T)$ is the well-konwn collision frequency, with $Z(T) = \pi {b_{\max}}^{2}\sqrt{(8k_{\mathrm{B}}T)/(\pi\mu)}$, where $b_{\max}$ is the maximum impact parameter and $\mu$ is the reduced mass of the collision partner, $f_{\mathrm{B}}(E_{\mathrm{col}}, T)$ is the distribution of the collisional energy $E_{\mathrm{col}}$ given by the normalized Boltzmann distribution at temperature $T$, with:

$$f_{\mathrm{B}}(E_{\mathrm{col}}, T) = \frac{E_{\mathrm{col}}}{(k_{\mathrm{B}}T)^{2}}\exp\left(-\frac{E_{\mathrm{col}}}{k_{\mathrm{B}}T}\right) \qquad (\mathrm{S2}-4)$$

For convenince, Eq. (S2-3) can be converted into the following form:

$$k(\upsilon' \rightarrow \upsilon,\, T) = Z(T)\phi(\upsilon' \rightarrow \upsilon,\, T) \qquad \text{(S2-5a)}$$

in which,

$$\phi(\upsilon' \rightarrow \upsilon,\, T) = \int_0^\infty P(\upsilon' \rightarrow \upsilon,\, E_{\mathrm{col}}) \cdot f_{\mathrm{B}}(E_{\mathrm{col}},\, T)dE_{\mathrm{col}} \qquad \text{(S2-5b)}$$

Here $\phi(\upsilon' \rightarrow \upsilon,\, T)$ is the thermal averaged state-to-state transition probability given by Eq. (S2-5b).

With the equations above, the state-to-state transition rate coefficients can be computed from the statistical results based on batches of trajectories. Notice, the rotational temperature $T_{\mathrm{r}}$ is equal to the transitional temperature $T$ for simplicity in the current work, which is based on the fact that rotational degrees of freedom (d.o.f) may relax with the transitional d.o.f rapidly [13,14].

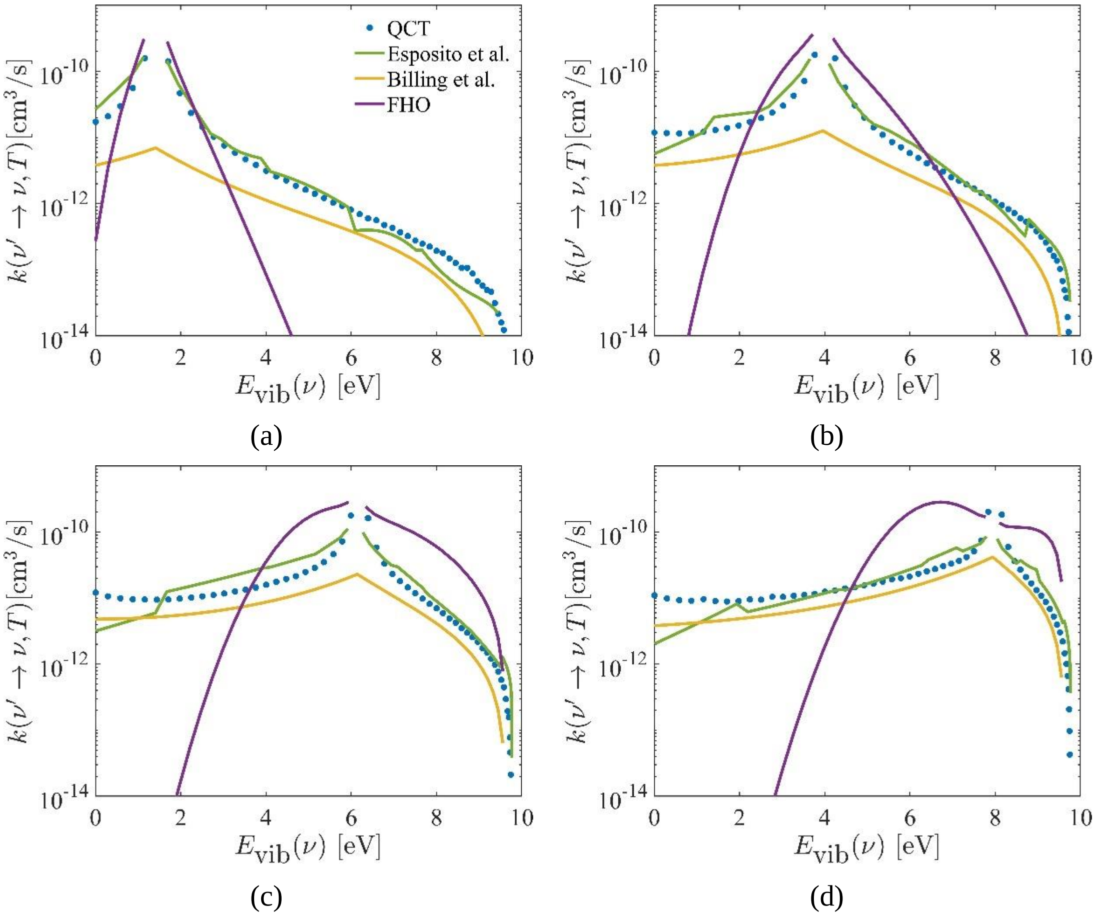


Fig.S1 State-to-state transition rates in $T$=20000 K from QCT simulation and comparison with Esposito et al.'s model, Billing et al.'s model, and FHO model. (a) From $\upsilon'$=05 initial vibrational state; (b) From $\upsilon'$=15 initial vibrational state; (c) From $\upsilon'$=25 initial vibrational state; (d) From $\upsilon'$=35 initial vibrational state.

The state-to-state transition rate coefficients at three temperatures $T$=10000 K, $T$=20000 K, and $T$=30000 K were calculated. Fig.S1 shows the our calculated transition rate coefficients (blue dots) , compared with three widely used models: forced harmonic oscillator (FHO) model [15,16] (purple lines), Billing et al.'s model [17] (yellow lines), and Esposito et al.'s model [9] (green lines). The calculation of

the FHO and Billing et al.'s model is implemented with the software Kinetic Approach to Physical Processes in Atmospheres (KAPPA) [18].

In general, our results agree well with Esposito et al.'s model, which is an empirical piecewise fitting containing several hundreds of parameters for accuracy, although the latter exhibits slight discontinuities in the piecewise positions. While Billing et al.'s empirical model effectively describes the qualitative aspects of the trends, it demonstrates some quantitative discrepancies. Clearly, the wide range of vibrational energy transfer is significant, and thus cannot be explained by theoretical models that consider only energy transfer between nearby states [19,20] or the popular empirical "exponential-down" (ED) model [21–23] as argued in the main text. The more sophisticated theoretical model FHO achieves qualitative improvement in the sense, but still deviates considerably from the data.

# 3. Semi-Analytical Model for Transition Rate Coefficients

In this section, we introduce some details of our proposed Activation-Saturation (AS) model. In subsection 3.1, the “activation-saturation”-like behavior of the transition probability with collision energy is introduced; in subsection 3.2, we provide the detailed derivation of rate coefficients calculation using the steepest descent integration; in subsection 3.3, the results of rate coefficients from AS model are shown and compared with original QCT data; in subsection 3.4, the consistent “activation saturation”-like behavior in other atom-diatom systems ($O+N_2$ and $O+O_2$) is demonstrated.

## 3.1 Activation-Saturation Model of the Transition Probability

Inspired by the Arrhenius form of reaction rate constants, the variation of transition probability $P(\Delta E, E_{\mathrm{col}})$ in the upward energy transfer as a function of the collision energy $E_{\mathrm{col}}$ could be described by the following empirical model:

$$P(\Delta E, E_{\mathrm{col}}) = A\frac{E_0}{\Delta E}\exp\left(-\left(\frac{\Delta E}{E_{\mathrm{col}}}\right)^n\left(\frac{E_0}{E_{\mathrm{col}}}\right)^m\right) \qquad (\mathrm{S3}-1)$$

where $A$ is a dimensionless constant, $E_0$ is an energy parameter of the system, $\Delta E$ behaves as an activation energy, and the exponents $n$ and $m$ determine how fast the activation changes to saturation. This form describes a typical “activation-saturation” behavior, as discussed in the main text. For our system, $n\sim m\sim 1.5$, $E_0\sim 10.0\mathrm{eV}$ and $A\sim 3.0\times 10^{-4}$ agrees very well with the QCT data, as shown in Fig.S2(a). In Fig.S2 (b), we use $\frac{E_{\mathrm{col}}}{\Delta E^{\frac{n}{n+m}}\cdot E_{\mathrm{col}}^{\frac{m}{n+m}}}$ as the dimensionless collisional energy, and $\frac{P\Delta E}{E_0}$ as the dimensionless probability, and it’s obvious that the data with different $v$ collapse well with Eq.(S3-1).

These four parameters above are determined from fitting the data of rotational ground state of $v'$=25, i.e. ($v'$=25 $j'$=30), however, the “activation” behavior remains same within different initial ro-vibrational states. To confirm that, the transition probability from initial states at ($v'$=25 $j'$=30) and ($v'$=25 $j'$=30) has been demonstrated in Fig. S2 (c-d), and from initial states at ($v'$=5 $j'$=0) and ($v'$=15 $j'$=0) has been demonstrated in Fig. S2 (e-f). It’s obvious to conclude the weak dependence of these four parameters on initial $v'$ and $j'$, especially $n$ and $m$.

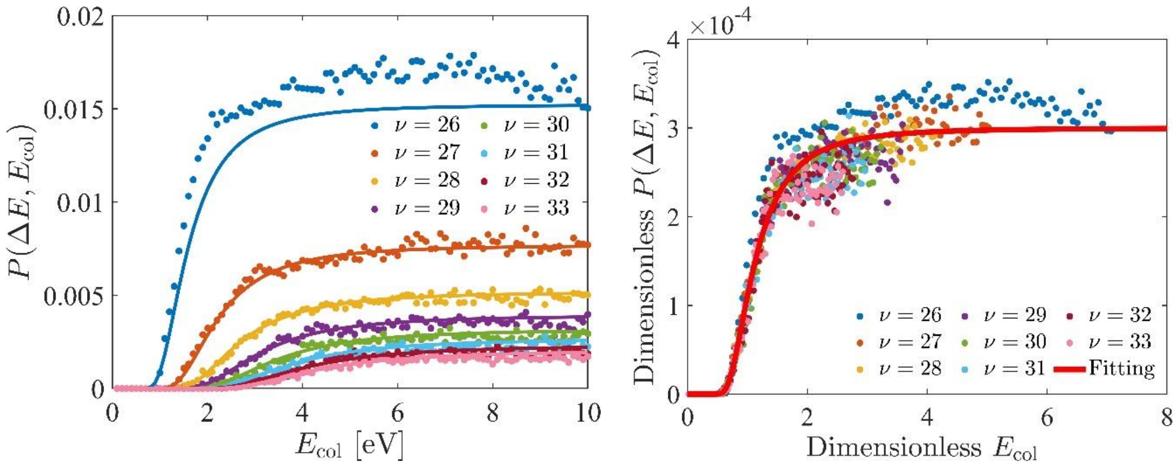


(a) (b)

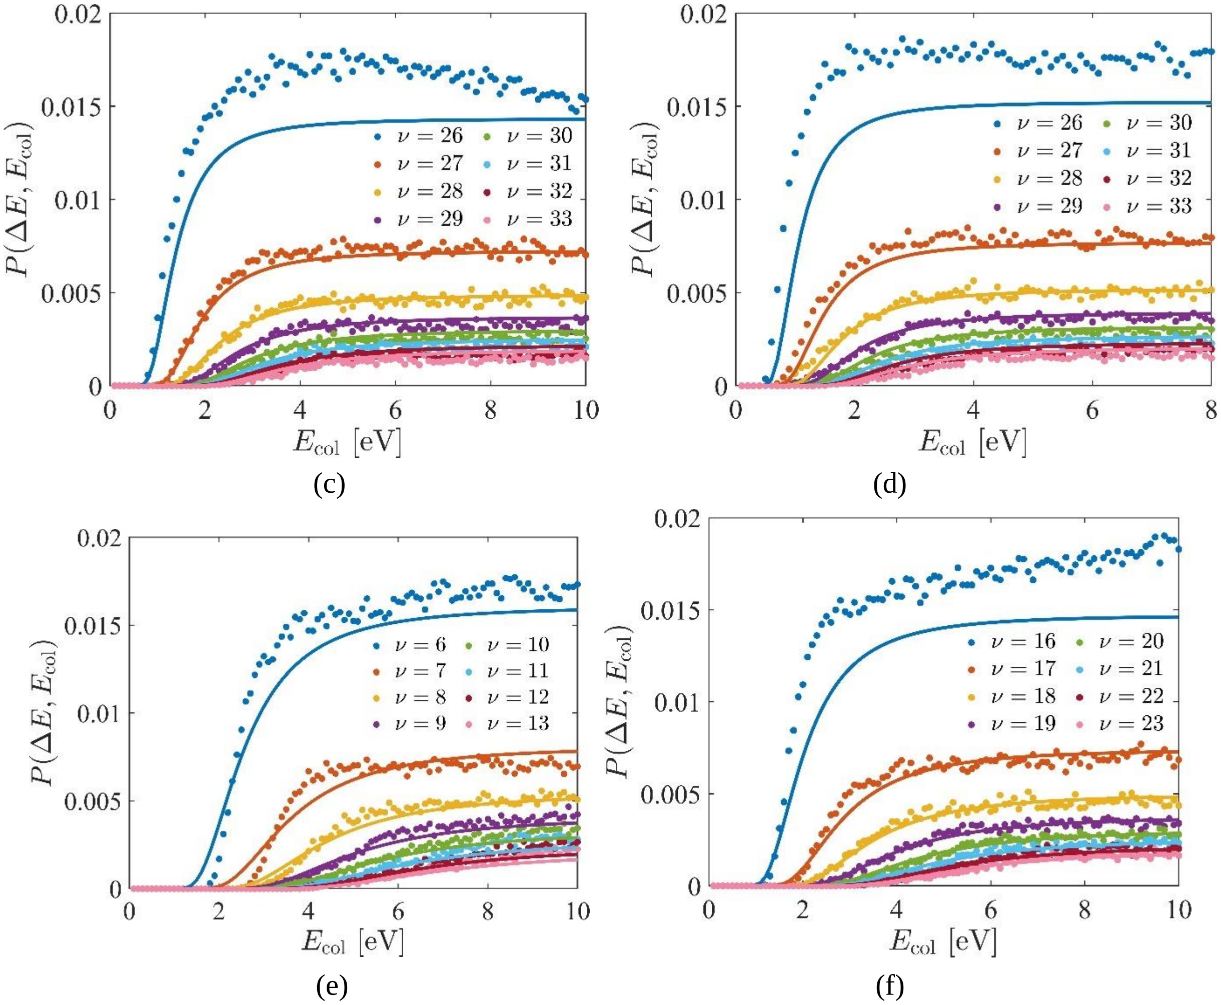


Fig.S2 State-to-state transition probability from the initial state at $\upsilon'$=25 with collision energy $E_{\mathrm{col}}$.
(a) Transition probability from QCT simulation (symbols) and fitting (solid lines), and the initial state is at ($\upsilon'$=25 $j'$=0); (b) Nondimensional transition probability with nondimensional collision energy and the fitting curve, and the initial state is at ($\upsilon'$=25 $j'$=0);
(c) initial state is at ($\upsilon'$=25 $j'$=30), and for this: $n\sim m\sim 1.5$, $E_0\sim 7.5$eV and $A\sim 3.8\times 10^{-4}$;
(d) initial state is at ($\upsilon'$=25 $j'$=60), and for this: $n\sim m\sim 1.5$, $E_0\sim 4.4$eV and $A\sim 6.8\times 10^{-4}$;
(e) initial state is at ($\upsilon'$=5 $j'$=0), and for this: $n\sim m\sim 1.5$, $E_0\sim 18.9$eV and $A\sim 2.3\times 10^{-4}$;
(f) initial state is at ($\upsilon'$=15 $j'$=0), and for this: $n\sim m\sim 1.5$, $E_0\sim 13.9$eV and $A\sim 2.5\times 10^{-4}$.

### 3.2 Steepest Descent Integration

It's not feasible to calculate the transition rate coefficient by just substituting eq.(S3-1) into eq.(S2-5) directly, because there's no analytic form for such integral. However, using the characteristics of the transition probability ($P(\Delta E, E_{\mathrm{col}})$ rises up to a plateau with $E_{\mathrm{col}}$) and the Boltzmann distribution ($F_{\mathrm{B}}(E_{\mathrm{col}}, T)$ decays exponentially with $E_{\mathrm{col}}$ at any given temperature $T$), the maximum of their product, corresponding to the so-called "most effective" collision energy, could be found. Then the "steepest descent integration" introduced by Landau [19], which is based on the fact that the integrand function is rapidly decreasing around this "most effective" collision energy, could be used to obtain the transition rate coefficient. In this subsection, the detailed derivation of the steepest descent integration is

introduced.

Here we focus on the thermal average transition probability $\phi(\Delta E,\, T)$, from which the transition rate coefficient can be obtained easily by multiplying it and the collision frequency. Substitute eq.(S3-1) into eq.(S2-5):

$$\begin{aligned}\phi(\Delta E,\, T) &= \int_0^\infty P(\Delta E, E_{\mathrm{col}}) \cdot \frac{E_{\mathrm{col}}}{k_{\mathrm{B}}T} \exp\left(-\frac{E_{\mathrm{col}}}{k_{\mathrm{B}}T}\right) \mathrm{d}\left(\frac{E_{\mathrm{col}}}{k_{\mathrm{B}}T}\right) \\ &= \int_0^\infty A \frac{E_0}{\Delta E} \exp\left(-\left(\frac{\Delta E}{E_{\mathrm{col}}}\right)^n \left(\frac{E_0}{E_{\mathrm{col}}}\right)^m\right) \cdot \frac{E_{\mathrm{col}}}{k_{\mathrm{B}}T} \exp\left(-\frac{E_{\mathrm{col}}}{k_{\mathrm{B}}T}\right) \mathrm{d}\left(\frac{E_{\mathrm{col}}}{k_{\mathrm{B}}T}\right) \qquad (\mathrm{S3}-2)\end{aligned}$$

In the main text, we stated that the asymptotic self-similar behavior of $k$ suggests that $k(v' \to v,\, T)$ depends on $\Delta E$ only, rather than $v'$ or $v$, thus $\Delta E$ appears as a variable instead of $v' \to v$. IF we define:

$$G(E_{\mathrm{col}}) = \left(\frac{\Delta E}{E_{\mathrm{col}}}\right)^n \left(\frac{E_0}{E_{\mathrm{col}}}\right)^m + \frac{E_{\mathrm{col}}}{k_{\mathrm{B}}T} \qquad (\mathrm{S3}-3)$$

Then, $\phi(\Delta E,\, T)$ can be written as

$$\phi(\Delta E,\, T) = \int_0^\infty A \frac{E_0}{\Delta E} \frac{E_{\mathrm{col}}}{(k_{\mathrm{B}}T)^2} \exp\big(-G(E_{\mathrm{col}})\big)\, dE_{\mathrm{col}} \qquad (\mathrm{S3}-4)$$

Set the first derivative of $G(E_{\mathrm{col}})$ to zero, the so-called "most effective" collision energy $E_{\mathrm{col}}^*$ is obtained:

$$G'(E_{\mathrm{col}}^*) = -(n+m) \frac{\Delta E^n {E_0}^m}{{E_{\mathrm{col}}^*}^{n+m+1}} + \frac{1}{k_{\mathrm{B}}T} = 0 \qquad (\mathrm{S3}-5)$$

which gives:

$$E_{\mathrm{col}}^* = \left[(n+m)\Delta E^n {E_0}^m k_{\mathrm{B}}T\right]^{\frac{1}{n+m+1}} \qquad (\mathrm{S3}-6)$$

and

$$G(E_{\mathrm{col}}^*) = \left(1 + \frac{1}{n+m}\right)(n+m)^{\frac{1}{n+m+1}} \left(\frac{\Delta E}{k_{\mathrm{B}}T}\right)^{\frac{n}{n+m+1}} \left(\frac{E_0}{k_{\mathrm{B}}T}\right)^{\frac{m}{n+m+1}} = \beta \eta^x \zeta^y \qquad (\mathrm{S3}-7)$$

where $\beta \equiv \left(1 + \frac{1}{n+m}\right)(n+m)^{\frac{1}{n+m+1}}$, $\eta \equiv \frac{\Delta E}{k_{\mathrm{B}}T}$, $\zeta \equiv \frac{E_0}{k_{\mathrm{B}}T}$, $x = \frac{n}{n+m+1}$, and $y = \frac{m}{n+m+1}$.

Next, expanding $G(E_{\mathrm{col}})$ at $E_{\mathrm{col}}^*$ in Taylor series:

$$G(E_{\mathrm{col}}) = G(E_{\mathrm{col}}^*) + \frac{G''(E_{\mathrm{col}}^*)}{2}(E_{\mathrm{col}} - E_{\mathrm{col}}^*)^2 + \cdots \qquad (\mathrm{S3}-8)$$

and substituting the expression into eq.(S3-4) yields

$$\phi(\Delta E,\, T) \cong A \frac{E_0}{\Delta E} \frac{\exp\left(-G(E_{\mathrm{col}}^*)\right)}{(k_{\mathrm{B}}T)^2} \int_0^\infty E_{\mathrm{col}} \exp\left(-\frac{G''(E_{\mathrm{col}}^*)}{2}(E_{\mathrm{col}} - E_{\mathrm{col}}^*)^2\right) dE_{\mathrm{col}} \qquad (\mathrm{S3}-9)$$

in which we neglected term of order high than $(E_{\mathrm{col}} - E_{\mathrm{col}}^*)^2$. Note that the second-order derivate of $G(E_{\mathrm{col}})$ at $E_{\mathrm{col}}^*$ is

$$G''(E_{\mathrm{col}}^*) = \frac{n+m+1}{E_{\mathrm{col}}^* \cdot k_{\mathrm{B}}T} = \frac{(n+m)F(E_{\mathrm{col}}^*)}{{E_{\mathrm{col}}^*}^2} \qquad (\mathrm{S3}-10)$$

Eq.(S3-9) can be evaluated approximately as

$$\phi(\Delta E,\,T)\cong A\frac{E_0}{\Delta E}\frac{\exp\left(-G(E_{\mathrm{col}}^*)\right)}{(k_\mathrm{B}T)^2}E_{\mathrm{col}}^*\sqrt{\frac{2\pi}{G''\left(E_{\mathrm{col}}^*\right)}}$$

$$\cong A[(n+m)]^{\frac{3}{2(n+m+1)}}\sqrt{\frac{2\pi}{n+m+1}}\left(\frac{\Delta E}{k_\mathrm{B}T}\right)^{\frac{3}{2}\frac{n}{n+m+1}-1}\left(\frac{E_0}{k_\mathrm{B}T}\right)^{\frac{3}{2}\frac{m}{n+m+1}+1}\exp\left(-G(E_{\mathrm{col}}^*)\right)$$

$$\cong \alpha\eta^{\frac{3}{2}x-1}\zeta^{\frac{3}{2}y+1}\exp(-\beta\eta^x\zeta^y) \qquad (\mathrm{S3}-11)$$

where $\alpha=A[(n+m)]^{\frac{3}{2(n+m+1)}}\sqrt{\frac{2\pi}{n+m+1}}$. Therefore, we have

$$k(\Delta E,\,T)=Z(T)\alpha\eta^{\frac{3}{2}x-1}\zeta^{\frac{3}{2}y+1}\exp(-\beta\eta^x\zeta^y) \qquad (\mathrm{S3}-12)$$

From eq.(S3-12), we can find the quantitative relationship of transition rate coefficient with the energy gap $\Delta E$ in the form of stretched exponential, $(\Delta E)^{\frac{n}{n+m+1}}$, which agrees with the observation from earlier experiments [24,25].

In Fig.S3, we plot the integrand in Eq.(S3-2), i.e., the transition probability times the exponential part of the Boltzmann distribution. The "most effective" collision energy is obvious in this figure, around which the integrand function decreases rapidly. Solid lines are the original function with QCT data, and dashed lines are the approximation of the integrand in the steepest descent integration.

Note that in the temperature cases ($T$ ~ $10^4$ K), the most contributed term in steepest descent integration, i.e. the "most effective" collision energy, may lie on the "activating" stage of the "activation-saturation" shape curve, which has been modeled with Eq.(S3-1) successfully. However, as the temperature decreasing ($T < 10^4$ K), the "most effective" collision energy may go closer to the "non-activating" stage, making the integration somewhat uncertain. Thus, this steepest descent integration is proved to be more reliable and accurate in the temperature cases ($T$ ~ $10^4$ K), which corresponds to the cases when wide range of vibrational energy transfer is significant.

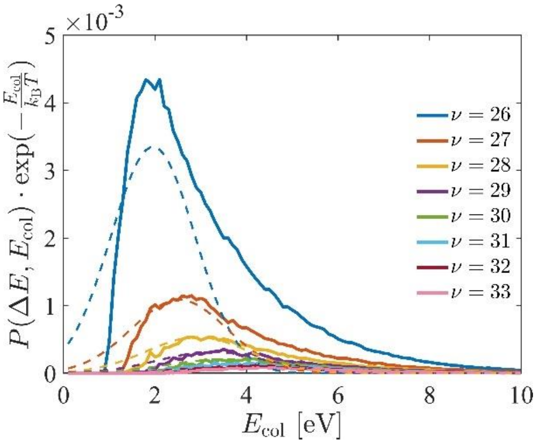


(a)

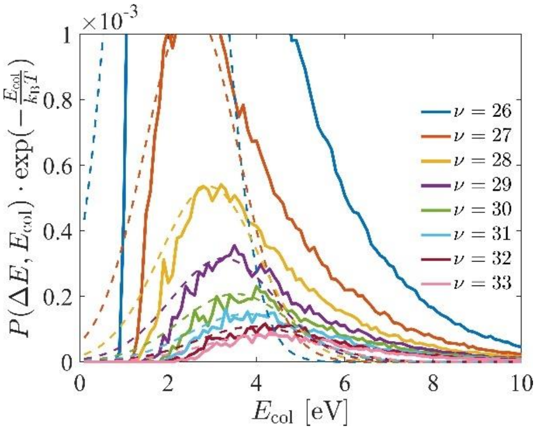


(b)

Fig.S3 State-to-state transition probability times the exponential part of the Boltzmann distribution in $T$= 20000K as a function of collisional energy. Panel (b) is a zoom in of panel (a). Solid lines are the original function with QCT data, and dashed lines are the approximation of the integrand in the steepest descent integration.

### 3.3 State-to-State Transition Rate Coefficients

We use the Eq.(S2-12) with $x = 3/8$, and $y = 3/8$ to determine the parameters $\alpha$ and $\beta$ from fitting the QCT simulation data in "upward" process, which gives $\alpha$ =0.0036 and $\beta$ =2.12. The "downward" process rates are calculated according to the detailed balance:

$$k(v' \to v, T) = \frac{\sum_0^{j_{\max}(v)}(2j+1)\exp\left(-\frac{E_{\text{int}}(v,j)}{k_B T}\right)}{\sum_0^{j_{\max}(v')}(2j'+1)\exp\left(-\frac{E_{\text{int}}(v',j')}{k_B T}\right)} k(v \to v', T) \quad (v' > v) \qquad (S3-13)$$

In our semi-analytical model, only two parameters $\alpha$ and $\beta$ are needed. One can either determine them from fitting the simulation data as mentioned above, or calculate them analytically with the relationship of $\alpha = A[(n+m)]^{\frac{3}{2(n+m+1)}}\sqrt{\frac{2\pi}{n+m+1}}$ and $\beta \equiv \left(1+\frac{1}{n+m}\right)(n+m)^{\frac{1}{n+m+1}}$, which gives $\alpha \approx$0.00057 and $\beta \approx$1.75. The fitting values and the analytical values are similar, however deviate with each other a little, which may come from the contribution of different initial rotational states or the uncertainty in modelling with Eq.(S3-1). Therefore, we use the fitting values for high accuracy. As shown in Fig. S4, the results from our semi-analytical model are in good agreement with the QCT data over a wide range of energy transfer and temperatures (especial when the temperature is high).

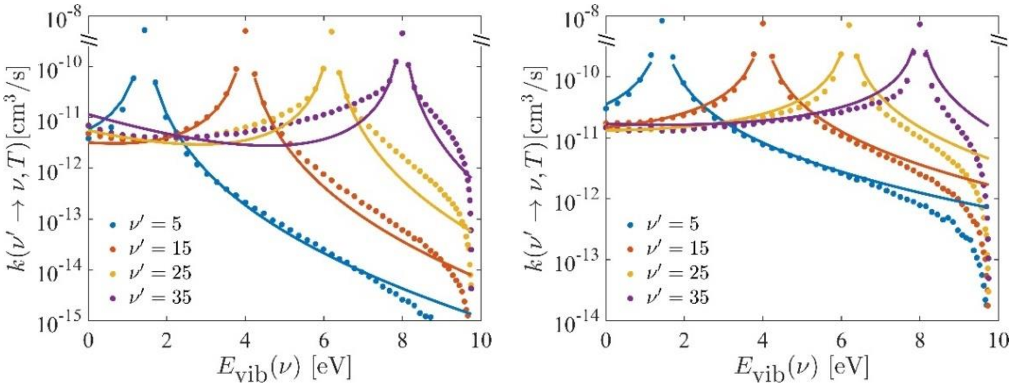


(a) (b)

Fig. S4. State-to-state transition rate at different temperatures as a function of the vibrational energy of the final state. Different colors indicate the transition rates from different initial vibrational energy states. Symbols are QCT data, and curves are results given by our semi-analytical model. (a) $T$ = 10000 K; (b) $T$ = 30000 K.

### 3.4 Consistent Behavior in Other Atom-Diatom Systems

Moreover, the AS model of the transition probability with the collisional energy is not only valid in the $N+N_2$ system, and we also found that there is a consistent behavior in the collision dynamics of $O+N_2$, and $O+O_2$, as shown in Fig.S5. Therefore, if the state-to-state rate coefficients of a specific new system are needed, one can first obtain these four parameters: $n$, $m$, $E_0$ and $A$, in "activation-saturation" curve with only a few simulation data, and then build the coefficients calculation model with Eq. S3-12

involving transitions among all states at high temperatures efficiently.

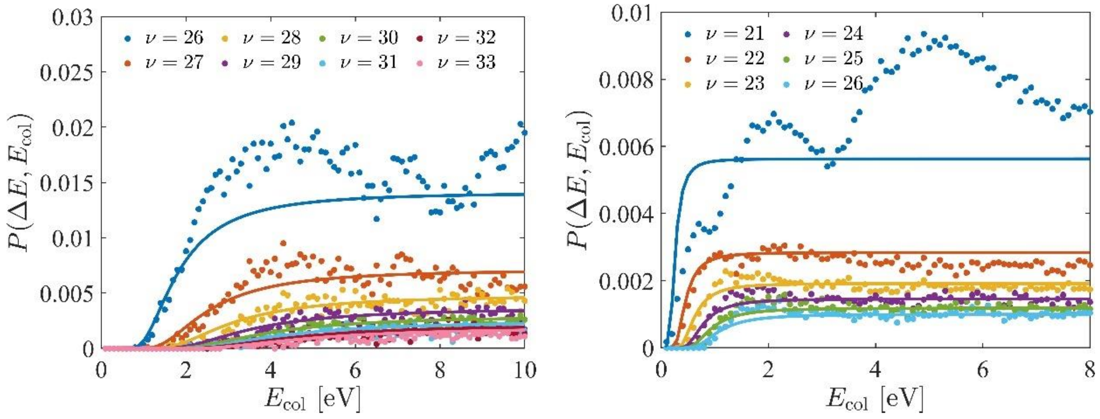


(a) (b)

Fig. S5. State-to-state transition probability and state-to-state transition rate of various atom-diatom collision systems.

(a) O+$N_2$ (initial state at ($v'$=25 $j'$=0), @$1^3A''$), $n{\sim}m{\sim}1.2$, $E_0{\sim}12.6$eV and $A{\sim}2.2\times10^{-4}$;

(b) O+$O_2$ (initial state at ($v'$=20 $j'$=0), @$1^3A''$), $n{\sim}2.5$, $m{\sim}0.5$, $E_0{\sim}3.2$eV and $A{\sim}3.5\times10^{-4}$.

# 4. Relaxation of N+$N_2$ after Passing a Shock in Hypersonic Flows

In this section, we use the master equation to simulate the vibrational energy relaxation of N+$N_2$ mimicking the gas behind strong shocks in a hypersonic flow.

Referring to Refs [26,27], the energy relaxation of N+$N_2$ can be considered occurring in an ideal isochoric and isothermal reactor maintained at a constant translational temperature $T$. The initial vibrational temperature $T_v$ corresponding to the temperature of the gas before encountering the shock is much lower than the fixed translational temperature. Energy transfer processes by $N_2$-$N_2$ collision is negligible with respect to the processes induced by N atom.

We focus on the vibrational energy transfer and neglect the dissociation, therefore, $N_2$ molecule and N atom maintain a constant number density in this process.

$$\mathrm{N}_2(v') + \mathrm{N} \leftrightarrow \mathrm{N}_2(v) + \mathrm{N} \qquad (\mathrm{S4}-1)$$

The time evolution of populations at vibrational state $v$ is described by the master equation:

$$\frac{dn_v}{dt} = n_\mathrm{N} \sum_{v' \neq v} [k(v' \to v,\, T) n_{v'} - k(v \to v',\, T) n_v] \qquad (\mathrm{S4}-2)$$

in which, $n_v$ is the number density at vibrational state $v$ of $N_2$ molecule, and $n_\mathrm{N}$ is the number density of N atom. The master equation could be written in a matrix form:

$$\frac{d[n_v]}{dt} = [M][n_v] \qquad (\mathrm{S4}-3a)$$

$$M_{vv'} = \begin{cases} n_\mathrm{N} \cdot k(v' \to v,\, T), & (v' \neq v) \\ -n_\mathrm{N} \cdot \sum_{v' \neq v} k(v \to v',\, T), & (v' = v) \end{cases} \qquad (\mathrm{S4}-3b)$$

in which, $[n_v]$ is the column vector form of the vibrational state population, and $[M]$ is the transition matrix constructed with the transition rate coefficients. With the eigenvalue analysis of $[M]$ matrix, the analytical solution is given as,

$$[n_v] = \sum_l \alpha_l \exp(\lambda_l t)\, [\overrightarrow{V_l}] \qquad (\mathrm{S4}-4)$$

Here, $\lambda_l$ and $[\overrightarrow{V_l}]$ are the eigenvalue and eigenvector of $[M]$ matrix. $\alpha_l$ is the coefficients determined by the initial condition,

$$[\alpha_l] = [V_l]^{-1} [n_v]_{t=0} \qquad (\mathrm{S4}-5)$$

With the population evolution, the average vibrational energy at a specific time could be obtained,

$$\langle E_\mathrm{vib} \rangle = \frac{\sum E_\mathrm{vib}(v) \cdot n_v}{\sum n_v} \qquad (\mathrm{S4}-6)$$

## 4.1 Relaxation of Vibrational Energy with Time

The first example refers to Ref [26], in which the number density of the gas is $2.4\times10^{18}$ $cm^{-3}$ and the molar fraction for N atom is 5%. Although the assumption of neglecting the $N_2$-$N_2$ collision is uncertain at such a low molar fraction for N atom, we still adopt the same setting enabling for comparison. The initial vibrational temperature $T_v$ is set to 300 K, and the translational temperatures are in range of $T \sim 10^4$ K. The rotational temperature $T_r$ of the gas in Ref [26] was assumed to vary simultaneously with the

vibrational temperature by solving ro-vibrational-state-resolved master equations, which is different from the treatment in our approach where $T_r = T$ is assumed. The difference, however, should be very small as it is known that the rotational d.o.f reaches equilibrium with the transnational d.o.f much earlier than the vibrational d.o.f [13,14].

In order to verify our proposed model, we calculate thermal relaxation and population distribution evolution compared with FHO model, Billing et al.'s model (Model B), and Esposito et al.'s model (Model E). The normalized vibrational energy $\langle E_{\text{vib}}(t)\rangle / \langle E_{\text{vib}}(t \to \infty)\rangle$ as a function of time is shown in Fig.S6 and Fig.4 in the main text. The AS model result is the closest to the benchmark given in Ref [26], comparable or slightly better than those from Esposito et al.'s model that contains several hundreds of fitting parameters, while Billing et al.'s model and the FHO model predict much slower relaxation of the vibrational energy.

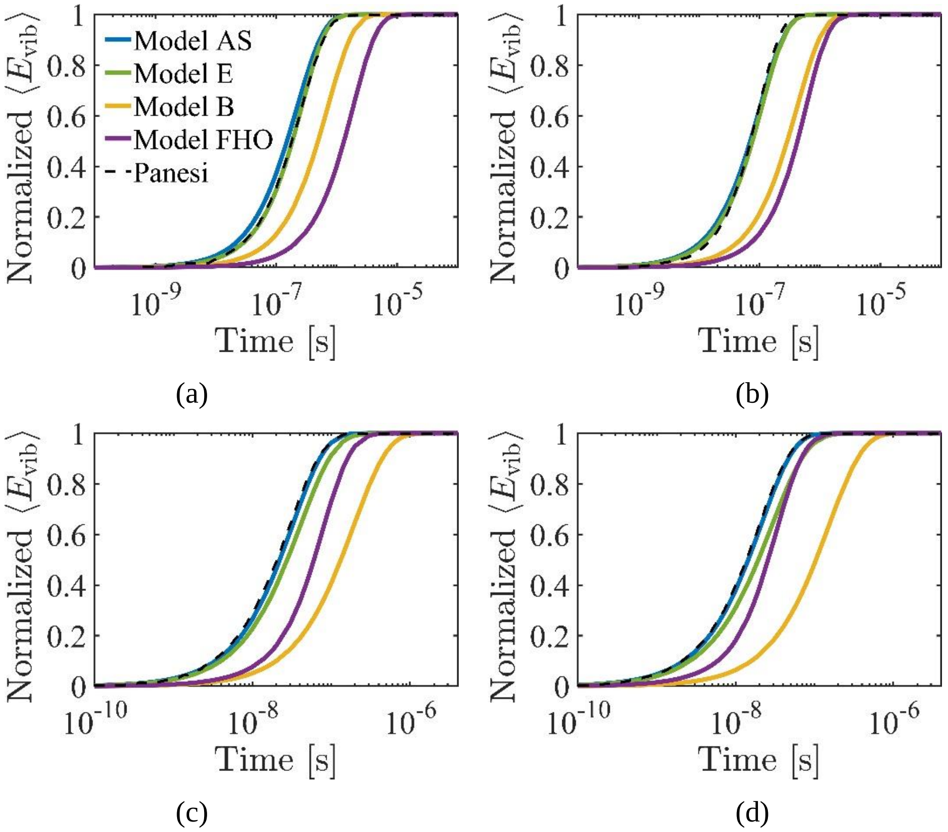


Fig.S6 The results of vibrational energy relaxation of a gas after passing a strong shock solved by master equation: (a) $T$=10000 K; (b) $T$=15000 K; (c) $T$=30000 K; (d) $T$=40000 K.

## 4.2 Vibrational Relaxation Time

The relaxation process is commonly characterized by the e-folding time $\tau$ [28] based on the approximation that $\frac{dE_{\text{vib}}(t)}{dt} \approx -\frac{E_{\text{vib}}(t)-E_{\text{inf}}}{\tau}$, where $E_{\text{inf}} = E_{\text{vib}}(t \to \infty)$, which yields $\frac{E_{\text{vib}}(t)-E_{\text{inf}}}{E_0-E_{\text{inf}}} \approx \exp\left(-\frac{t}{\tau}\right)$ with $E_0 = E_{\text{vib}}(t = 0)$. Figure S7(a) shows that the dependence of $\frac{E_{\text{vib}}(t)-E_{\text{inf}}}{E_0-E_{\text{inf}}}$ on time $t$ from our master equation results follows the exponential decay very well, and the relaxation time $\tau$ can

be obtained from $\frac{E_{\text{vib}}(t)-E_{\text{inf}}}{E_0-E_{\text{inf}}} = \exp(-1) \approx 0.368$.

For the relaxation time, based on an empirical equation by Millikan and White [29], Park proposed a model [30] that has the form of $\ln(\tau p) \sim aT^{-\frac{1}{3}} - b$, where $p$ is the partial pressure of bath gas (N atom in current work), $a$ and $b$ are parameters fitted from experimental data with $a$ describing the dependence of $\tau$ on $T^{-\frac{1}{3}}$ and $b$ determining the magnitude of the relaxation time as Park's model can be written as $\tau \sim \frac{1}{pe^b}\exp(aT^{-\frac{1}{3}})$. In Fig. 4(b) of the main text, the e-folding time obtained from our results is plotted as a function of $T^{-\frac{1}{3}}$, together with Park's model [30], and some simulation results including Panesi et al.'s master equation (ME) results [26], Kim et al.'s ME results in Ref [27], Macdonald et al.'s ME results in Ref [31], and Macdonald et al.'s direct molecular simulation (DMS) results in Ref [31]. The ME study in Ref [26] was based on the state-to-state transition rate coefficients carefully tabulated in the NASA database [32], Kim et al.'s used bound-to-bound transition rate coefficients of the same database to carry ME investigation, and in a more recent work [31] the ME study is based on an updated version of this database with higher accuracy. DMS method can resolve the relaxation process by directly simulating quasi-classical trajectories based on the framework of DSMC [31,33]. Note that we carried master equation investigation only for the cases with relatively high temperatures ($T \geqslant 10000$ K), when the wide range of vibrational energy transfer is significant enabling our proposed model adequate, as discussed before.

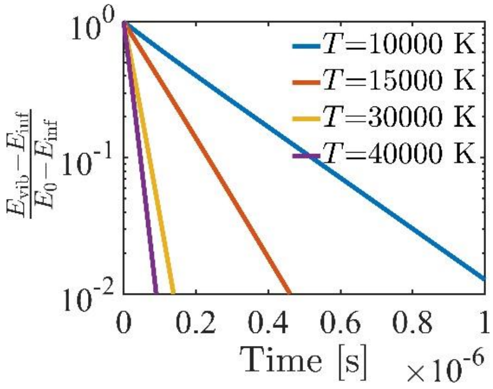


(a)

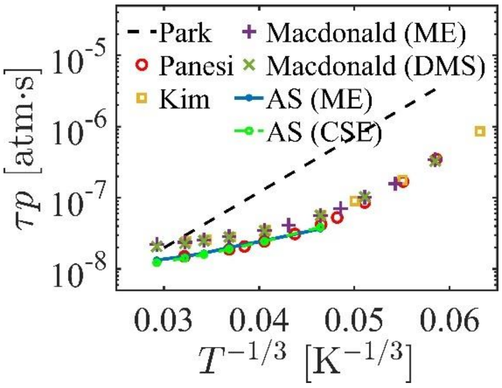


(b)

Fig.S7 The vibrational relaxation time. (a) The normalized vibrational energy $\frac{E_{\text{vib}}(t)-E_{\text{inf}}}{E_0-E_{\text{inf}}}$ in logarithmic scales as a function of time. (b) Change of the e-folding time $\tau$ with the translational temperature $T$.

The comparison suggests that Park's model captures the trends, however the value of $a$ and $b$ may differ in the high and low temperature range separately. In the low-temperature range, the slope $a$ in the original Park's model is consistent with the slope given by the simulation results, which is not surprising as the parameters in Park's model are extracted from the experimental data at $T \leqslant 8000$ K. The discrepancy in $b$ between Park's model and the simulation results comes possibly from the uncertainties in

the experimental data and/or the limitation of the simulation method at low temperatures. In the high-temperature range, our results are satisfactory within a factor of two of available simulation results from Refs [26,27,31], and especially are in good agreement with Panesi et al.'s results [26]. The discrepancy can be mainly attributed to our simplified treatment of rotational energy, rather than the uncertainty of our proposed model. In our investigation, the rotational energy is assumed to be always equilibrated with translational energy, however, the relaxation of rotational energy is resolved together with vibrational energy in Refs [26,27,31]. While the rotation-vibration coupling has been found more significant at high temperature cases [26,27,31]. Therefore, the neglect of rotational relaxation at high temperatures will accelerate the relaxation process, resulting in a deviation in relaxation time. Understanding the rotational energy transfer behavior in the future is helpful to build a more comprehensive model resolving the both rotational and vibrational states, enabling us to obtain more accurate results on the relaxation time. The dependence of $\ln(\tau)$ on $T^{-\frac{1}{3}}$ can also be described by Park's model, but with a different slope $a$. The AS model proposed in this work could shed light on how to determine the slope $a$ in this temperature regime.

Furthermore, here we provide an analytical way to obtain the relaxation time. With our proposed AS model, the transition matrix in Eq. S4-3b can be constructed easily. According to the chemically significant eigenmodes (CSE) theory [34], the eigenvalues of the transition matrix can be used to characterize the rate of the energy relaxation in this case. The smallest eigenvalue is zero, whose eigenvector corresponds to the final-state equilibrium distribution. The second smallest eigenvalue, i.e., the minimum eigenvalue other than zero, whose reciprocal is the time that characterizes the rate of energy relaxation. Figure S7 shows that the e-folding time obtained from the master equation results (AS Model ME) and the relaxation time from the CSE theory (AS Model CSE) agree well with each other.

## 4.3 Vibrational Energy Distribution

For more details, the evolution of vibrational energy distribution solved by our AS model and Esposito et al.'s model is compared in Fig.S8. Population distribution with these two models is consistent in low energy states. However, because complex and piecewise fitting forms are used in Esposito et al.'s model as seen in Fig.S1, the distribution looks a little discontinuous.

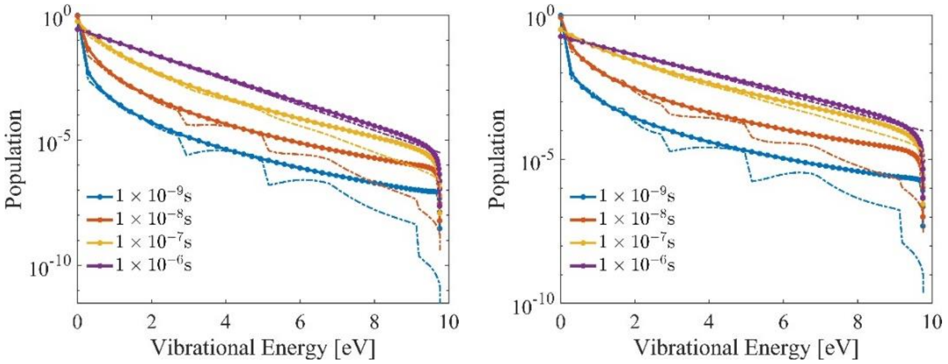


(a) (b)

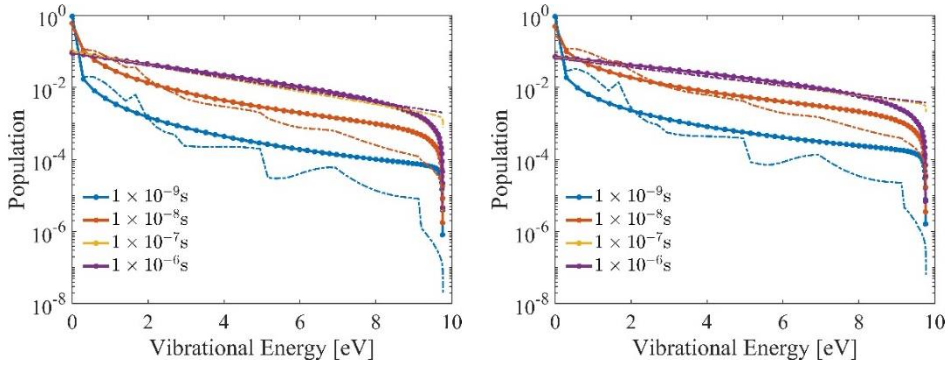


(c) (d)

Fig.S8 Vibrational states distribution evolution behind shock wave in hypersonic flow solved by master equation (solid line for our proposed model, dashed line for Esposito et al.'s model) (a) *T*=10000 K (b) *T*=15000 K (c) *T*=30000 K (d) *T*=40000 K

There is another simulation example in Ref [27], where the number density of the $N_2$ molecule and N atom is $5\times10^{18}$ $cm^{-3}$ and the initial temperature is 1000 K. Fig.S9(a) shows the comparison of vibrational energy relaxation from Ref [27] with our proposed model. Our model gives a slower relaxation process compared with Kim et al.'s result, because only bound-to-bound transition is considered in their calculation. However, quasi-bound states occur mostly in high energy states, which need a long time to equilibrate. Vibrational energy distribution evolution is shown is Fig.S9(b). The population of the first few states agrees well, and the main discrepancy occurs at the high energy states. The lower "tail" is obvious in their result, which is also because the transitions from bound states to quasi-bound states are neglected in Ref [27].

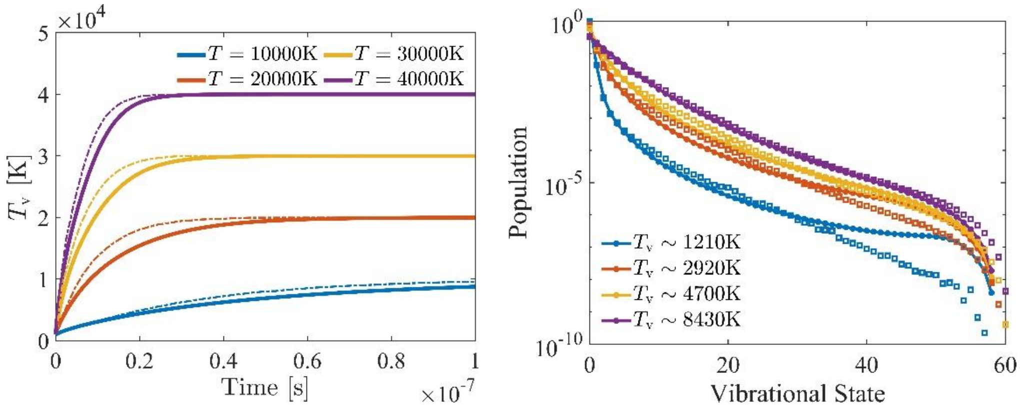


(a) (b)

Fig.S9 Thermal relaxation and vibrational states distribution evolution behind shock wave in hypersonic flow solved by master equation. (a) Thermal relaxation in four different translational temperatures (solid line for our proposed model, dashed line for Kim et al.'s result); (b) Vibrational states distribution evolution in *T*=10000 K at four moment (solid line for our proposed model, square for Kim et al.'s result)

In summary, the observed "activation-saturation" (AS) like behavior of the transition probability with the collisional energy leads to a step forward in the understanding of vibrational energy transfer, which leads to a physics-based semi-analytical model for calculating the state-to-state transition rate coefficients. Furtherly, with our proposed AS model, the vibrational energy relaxation in the $N+N_2$

system mimicking the gas behind strong shocks in a hypersonic flow is investigated using master equation approach. The results of vibrational energy change, relaxation time, and population distribution are in good agreement with available data. Furthermore, it is interesting to investigate whether the same behavior can be observed in systems allowing non-adiabatic collisions, such as $O+O_2$ that possess multiple electronic states.

**Reference:**


[1] D. G. Truhlar and J. T. Muckerman, *Reactive Scattering Cross Sections III: Quasiclassical and Semiclassical Methods*, in *Atom - Molecule Collision Theory* (Springer US, Boston, MA, 1979), pp. 505–566.

[2] N. C. Blais and D. G. Truhlar, *Monte Carlo Trajectory Study of Ar + $H_2$ Collisions. I. Potential Energy Surface and Cross Sections for Dissociation, Recombination, and Inelastic Scattering*, J. Chem. Phys. **65**, 5335 (1976).

[3] J. D. Bender, P. Valentini, I. Nompelis, Y. Paukku, Z. Varga, D. G. Truhlar, T. Schwartzentruber, and G. V. Candler, *An Improved Potential Energy Surface and Multi-Temperature Quasiclassical Trajectory Calculations of $N_2$ + $N_2$ Dissociation Reactions*, J. Chem. Phys. **143**, 054304 (2015).

[4] G. Czakó and J. M. Bowman, *Dynamics of the Reaction of Methane with Chlorine Atom on an Accurate Potential Energy Surface*, Science (80-. ). **334**, 343 (2011).

[5] R. Yin and B. Jiang, *Mechanical Vibrational Relaxation of NO Scattering from Metal and Insulator Surfaces: When and Why They Are Different*, Phys. Rev. Lett. **126**, 156101 (2021).

[6] Z. Varga and D. G. Truhlar, *Potential Energy Surface for High-Energy N + $N_2$ Collisions*, Phys. Chem. Chem. Phys. **23**, 26273 (2021).

[7] W. Lin, Z. Varga, G. Song, Y. Paukku, and D. G. Truhlar, *Global Triplet Potential Energy Surfaces for the $N_2$(X 1Σ) + O(3 P) → NO(X 2Π) + N(4 S) Reaction*, J. Chem. Phys. **144**, (2016).

[8] Z. Varga, Y. Paukku, and D. G. Truhlar, *Potential Energy Surfaces for O + $O_2$ Collisions*, J. Chem. Phys. **147**, (2017).

[9] F. Esposito, I. Armenise, and M. Capitelli, *N–$N_2$ State to State Vibrational-Relaxation and Dissociation Rates Based on Quasiclassical Calculations*, Chem. Phys. **331**, 1 (2006).

[10] F. Esposito, I. Armenise, G. Capitta, and M. Capitelli, *O-$O_2$ State-to-State Vibrational Relaxation and Dissociation Rates Based on Quasiclassical Calculations*, Chem. Phys. **351**, 91 (2008).

[11] P. Valentini, T. E. Schwartzentruber, J. D. Bender, I. Nompelis, and G. V. Candler, *Direct Molecular Simulation of Nitrogen Dissociation Based on an Ab Initio Potential Energy Surface*, Phys. Fluids **27**, 086102 (2015).

[12] Y. Shu, L. Zhang, and D. G. Truhlar, *ANT 2023: A Program for Adiabatic and Nonadiabatic Trajectories*, Comput. Phys. Commun. **296**, 109021 (2024).

[13] G. Colonna, I. Armenise, D. Bruno, and M. Capitelli, *Reduction of State-to-State Kinetics to Macroscopic Models in Hypersonic Flows*, J. Thermophys. Heat Transf. **20**, 477 (2006).

[14] G. V. Candler, *Rate Effects in Hypersonic Flows*, Annu. Rev. Fluid Mech. **51**, 379 (2019).

[15] E. H. Kerner, *Note on the Forced and Damped Oscillator in Quantum Mechanics*, Can. J. Phys. **36**, 371 (1958).

[16] I. V. Adamovich, S. O. Macheret, J. W. Rich, and C. E. Treanor, *Vibrational Energy Transfer Rates Using a Forced Harmonic Oscillator Model*, J. Thermophys. Heat Transf. **12**, 57 (1998).

[17] G. D. Billing and E. R. Fisher, *VV and VT Rate Coefficients in $N_2$ by a Quantum-Classical Model*, Chem. Phys. **43**, 395 (1979).

[18] L. Campoli, G. P. Oblapenko, and E. V. Kustova, *Overview and Perspectives of KAPPA Library*, AIP Conf. Proc. **2132**, (2019).

[19] L. D. Landau, *Theory of Sound Dispersion*, Phys. Zeitschrift Der Sowjetunion **10**, 34 (1936).

[20] R. N. Schwartz, Z. I. Slawsky, and K. F. Herzfeld, *Calculation of Vibrational Relaxation Times in*

*Gases*, J. Chem. Phys. **20**, 1591 (1952).

[21] I. Oref and D. C. Tardy, *Energy Transfer in Highly Excited Large Polyatomic Molecules*, Chem. Rev. **90**, 1407 (1990).

[22] J. R. Barker, L. M. Yoder, and K. D. King, *Vibrational Energy Transfer Modeling of Nonequilibrium Polyatomic Reaction Systems*, J. Phys. Chem. A **105**, 796 (2001).

[23] A. W. Jasper, K. M. Pelzer, J. A. Miller, E. Kamarchik, L. B. Harding, and S. J. Klippenstein, *Predictive a Priori Pressure-Dependent Kinetics*, Science (80-. ). **346**, 1212 (2014).

[24] U. Hold, T. Lenzer, K. Luther, K. Reihs, and A. C. Symonds, *Collisional Energy Transfer Probabilities of Highly Excited Molecules from Kinetically Controlled Selective Ionization (KCSI). I. The KCSI Technique: Experimental Approach for the Determination of P(E',E) in the Quasicontinuous Energy Range*, J. Chem. Phys. **112**, 4076 (2000).

[25] T. Lenzer, K. Luther, K. Reihs, and A. C. Symonds, *Collisional Energy Transfer Probabilities of Highly Excited Molecules from Kinetically Controlled Selective Ionization (KCSI). II. The Collisional Relaxation of Toluene: P(E',E) and Moments of Energy Transfer for Energies up to 50 000 Cm −1*, J. Chem. Phys. **112**, 4090 (2000).

[26] M. Panesi, R. L. Jaffe, D. W. Schwenke, and T. E. Magin, *Rovibrational Internal Energy Transfer and Dissociation of $N_2$(1Σg+)−N(4Su) System in Hypersonic Flows*, J. Chem. Phys. **138**, 044312 (2013).

[27] J. G. Kim and I. D. Boyd, *State-Resolved Master Equation Analysis of Thermochemical Nonequilibrium of Nitrogen*, Chem. Phys. **415**, 237 (2013).

[28] C. Park, *Rotational Relaxation of N2 behind a Strong Shock Wave*, J. Thermophys. Heat Transf. **18**, 527 (2004).

[29] R. C. Millikan and D. R. White, *Systematics of Vibrational Relaxation*, J. Chem. Phys. **39**, 3209 (1963).

[30] C. Park, *Review of Chemical-Kinetic Problems of Future NASA Missions, I: Earth Entries*, J. Thermophys. Heat Transf. **7**, 385 (1993).

[31] R. L. Macdonald, E. Torres, T. E. Schwartzentruber, and M. Panesi, *State-to-State Master Equation and Direct Molecular Simulation Study of Energy Transfer and Dissociation for the $N_2$ – N System*, J. Phys. Chem. A **124**, 6986 (2020).

[32] R. Jaffe, D. Schwenke, and G. Chaban, *Vibrational and Rotational Excitation and Dissociation in $N_2$-$N_2$ Collisions from Accurate Theoretical Calculations*, in *10th AIAA/ASME Joint Thermophysics and Heat Transfer Conference* (American Institute of Aeronautics and Astronautics, Reston, Virigina, 2010), pp. 1–13.

[33] P. Valentini, T. E. Schwartzentruber, J. D. Bender, and G. V. Candler, *Dynamics of Nitrogen Dissociation from Direct Molecular Simulation*, Phys. Rev. Fluids **1**, 043402 (2016).

[34] J. T. Bartis and B. Widom, *Stochastic Models of the Interconversion of Three or More Chemical Species*, J. Chem. Phys. **60**, 3474 (1974).
